# Supplementary material for: Direct Post-Training Preference Alignment for Multi-Agent Motion Generation Models Using Implicit Feedback from Pre-training Demonstrations
Source: arXiv:2503.20105 source file (2025-03-25)
Supplement: Supplementary file 1 [file appendix.tex]

\section{Appendix}
\label{app:appendix}

\input{sections/releated_work}

\subsection{Optimal Transport Based Reward}
\label{app:OT}

\textbf{Setup.} Let $\obstraj = \{\obs^t\}_{t=1}^{t=T}$ be a trajectory of observations, where $T$ is the trajectory length. Let $\mathcal{D}_+ \subset \mathcal{S}_{\reph}$ be a dataset of preferred videos from the preference video dataset and $\mathcal{D}_\robot$ be the set of videos induced by a given robot policy $\policyr$. 
We denote $\phi: \mathbb{R}^{h,w,3} \rightarrow \mathbb{R}^{n_e}$ as an observation encoder that maps a $h \times w$ RGB image to a $n_e$ dimensional embedding. 
For any video $\obstraj$, let the induced empirical embedding distribution be $\rho = \frac{1}{T} \sum_{t=0}^{T} \delta_{\repr(\obs^t)}$, where $\delta_{\repr(\obs^t)}$ is a Dirac distribution centered on $\repr(\obs^t)$. 

% For a video $\obstraj_+ \in \mathcal{D}_+$, let $\rho_+$ be its empirical embedding distribution, and for $\obstraj_R \in \mathcal{D}_\robot$ let $\rho_\robot$ be the corresponding embedding distribution. 

\textbf{Background.} 
Optimal transport finds the optimal coupling $\mu^* \in \mathbb{R}^{T \times T}$ that transports the robot embedding distribution, $\rho_\robot$, of a robot video $\obstraj_\robot \in \mathcal{D}_\robot$ to the expert video embedding distribution, $\rho_+$ for $\obstraj_+ \in \mathcal{D}_+$, with minimal cost (as measured by a distance function, e.g. cosine distance). This comes down to an optimization problem that minimizes the Wasserstein distance between the two distributions: 
\begin{equation}
\begin{aligned}
\mu^{*} = \argmin_{\mu \in \mathcal{M}(\rho_\robot, \rho_+)} \sum_{t=1}^{T}\sum_{t'=1}^{T} c\big(\phi(\obs^t_\robot), \phi(\obs^{t'}_+)\big)\mu_{t,t'}.
\end{aligned}
\label{eq:app_ot_problem}
\end{equation}
where $\mathcal{M}(\rho_\robot, \rho_+) = \{\mu \in \mathbb{R}^{T \times T}: \mu\mathbf{1} = \rho_{\mathrm{R}}, \mu^{T}\mathbf{1} = \rho_+\}$ is the set of coupling matrices and $c: \mathbb{R}^{n_\robot} \times \mathbb{R}^{n_+}\rightarrow \mathbb{R}$ is a cost function defined in the embedding space (e.g., cosine distance). The optimal transport plan gives rise to the following reward signal that incentivizes the robot to stay within the expert demonstration distribution by explicitly minimizing the distance between the observation distribution and expert distribution:
\begin{equation}
\begin{aligned}
\rewr(\obs^t_\mathrm{R}; \repr) = -\sum_{t'=1}^{T} c\big(\repr(\obs^{t}_\robot), \repr(\obs^{t'}_+)\big)\mu^{*}_{t, t'}.
\label{eq:app_ot_reward}
\end{aligned}
\end{equation}
    
\textbf{Regularized optimal transport.} Solving the above optimization in \autoref{eq:app_ot_problem} exactly is generally intractable for high dimensional distributions. In practice, we solve a entropy regularized version of the problem following the Sinkhorn algorithm \citep{peyre2019computational} which is %convex in $\mu$ and 
amenable to fast optimization:
\begin{equation}
    \begin{aligned}
    \mu^{*} = \argmin_{\mu \in \mathcal{M}(\rho_\robot, \rho_+)} \sum_{t=1}^{T}\sum_{t'=1}^{T} c\big(\phi(\obs^t_\robot), \phi(\obs^t_+)\big)\mu_{t,t'} - \epsilon\mathcal{H}(\mu),
    \end{aligned}
\label{eq:app_ot_problem_regu}
\end{equation}
where $\mathcal{H}$ denotes the entropy term that regularizes the optimization and $\epsilon$ is the associated weight. 

\textbf{Choosing an $\obstraj_+$ to match with $\policyr$.} The reward \eqref{eq:app_ot_reward} requires matching the robot to an expert observation video. To choose this expert observation, we follow the approach from \citep{haldar2023watch}. 
During policy optimization, given a robot's trajectory's observation $\obstraj_\mathrm{R}$ induced by the robot policy $\policyr$, we select the the ``closest" expert demonstration $\obstraj^*_+ \in \mathcal{D}_+$ to match the robot behavior with. This demonstration selection happens via:
\begin{equation}
\begin{aligned}
\obstraj^*_+ = \argmin_{\obstraj+ \in \mathcal{D_+}} \min_{\mu \in \mathcal{M}(\rho_\robot, \rho_+)} \sum_{t=1}^{T}\sum_{t'=1}^{T} c\big(\phi(\obs^t_\robot), \phi(\obs^{t'}_+)\big)\mu_{t,t'}.
\end{aligned}
\label{eq:select_expert_obs}
\end{equation}



\begin{figure}[h]
    \centering
    \includegraphics[width=\textwidth]{figs/attention_map.png}
    \caption{\textbf{Manipulation: Attention Map.} Visualization of attention map for RLHF-150 demos, RLHF-300 demos, and RAPL with 150 demos for both Franka and Kuka (cross-embodiment) images. Each entry of the figure shows two image snapshots from the relevant demonstration set with the attention map overlaid. Bright yellow areas indicate image patches that contribute most to the final embedding; darker purple patches indicate less contribution. $\phi_{RLHF-150}$ is biased towards paying attention to irrelevant areas that can induce spurious correlations; in contrast RAPL learns to focus on the task-relevant objects and the goal region. $\phi_{RLHF-300}$'s attention is slightly shifted to objects while still pays high attention to the robot embodiment.}
    \label{fig:attention_map}
\end{figure}

\rb{\subsection{Attention Map for \rapl and \rlhf}

In Figure~\ref{fig:attention_map} we visualize the attention map with a novel use of \textit{linear permutation} and \textit{kernel inflation} \citep{xu2022image2point}. Specifically, we use channel-averaged 2D feature map (\textit{i.e.,} activation map) as our attention map \citep{xu2020squeezesegv3}. Different from previous works that operate 2D feature maps, our approach utilizes a linear mapping $\mathcal{W} \in \mathcal{R}^{C_{in} \times C_{out}}$ on a 1D feature, which is average-pooled from a 2D feature $\mathcal{F}_{2D} \in \mathcal{R}^{C_{in} \times H \times W}$. Mathematically, the procedure can be formulated as
\begin{equation}
    \hat{\mathcal{F}}_{1D} = \frac{\mathcal{W}^T \times \sum_i^{H \times W}\mathcal{F}_{2D}^i}{H \times W}
\end{equation}
where $\hat{\mathcal{F}}_{1D} \in \mathcal{R}^{C_{out} \times 1}$ is the aligned features from our proposed RAPL by $\mathcal{W} \in \mathcal{R}^{C_{in} \times C_{out}}$. Inspired by \cite{xu2022image2point}, we can inflate the 1D linear mapping $\mathcal{W} \in \mathcal{R}^{C_{in} \times C_{out}}$ into 2D and keep the kernel size as 1, \textit{i.e.}, $\mathcal{W} \in \mathcal{R}^{C_{in} \times C_{out}} \rightarrow \mathcal{W}_{inflate} \in \mathcal{R}^{C_{in} \times C_{out} \times 1 \times 1}$. Then above equation can be equally represented as 
\begin{equation}
     \hat{\mathcal{F}}_{2D}  = \mathcal{W}_{inflate}^T \times \mathcal{F}_{2D}, 
     \hat{\mathcal{F}}_{1D} = \frac{\sum_i^{H \times W}\hat{\mathcal{F}}^i_{2D}}{H \times W}
\end{equation}
We average the $\hat{\mathcal{F}}_{2D} \in \mathcal{R}^{C_{out} \times H \times W}$ in channel dimension, and visualize the output as our attention map. A visualization of the full process is shown in Figure~\ref{fig:attention_map_method}.}

\begin{figure}[h]
    \centering
    \includegraphics[width=\textwidth]{figs/attention_map_method.png}
    \caption{\rb{\textbf{Attention Map Visualization Method.} (top) Visualization of our RAPL architecture. (bottom) Visualization of our process for creating a 2D attention map.} }
    \label{fig:attention_map_method}
\end{figure}



\subsection{Additional RLHF results: Ablation on Feedback Dataset Size}
\label{app:rlhf-with-doubled-data}

\begin{wrapfigure}{r}{0.4\textwidth}
    \vspace{-0.0cm} 
    \includegraphics[width=0.4\textwidth]{figs/franka_rlhf_double_data.png}
    \vspace{-0.5cm}
    \caption{\textbf{Manipulation.} \rapl outperforms \rlhf by $75\%$ with $50\%$ less training data.}
    \label{fig:rlhf_double_datasize}
    \vspace{-0.5cm}
\end{wrapfigure}
%
In Section~\ref{subsec:in-domain-manipulation}, it's surprising that \rlhf fails to learn a robot policy in a more realistic environment since its objective is similar to ours, but without explicitly considering representation alignment.  To further investigate this, we apply a linear probe on the final embedding and visualize the image heatmap of what \rapl's (our representation model trained with 150 training samples), \rlhf-150's (\rlhf trained with 150 samples), and \rlhf-300's (\rlhf trained with 300 samples samples) final embedding pays attention to in Figure~\ref{fig:attention_map}. 


We see that $\phi_{RAPL}$ learns to focus on the objects, the contact region, and the goal region while paying less attention to the robot arm;
$\phi_{RLHF-150}$ is biased towards
paying attention to irrelevant areas
that can induce spurious correlations (such as the robot arm and background area);
$\phi_{RLHF-300}$'s attention is slightly shifted to objects while still pays high attention to the robot embodiment.


When deploying $\phi_{RLHF-300}$ in Franka manipulation policy learning, we observe that policy performance is slightly improved (indicating that with more feedback data, preference-based reward prediction could yield to an aligned policy), but \rapl still outperforms \rlhf by $75\%$ with $50\%$ less training data, supporting the hypothesis: \textit{\rapl outperforms \rlhf with lower amounts of human preference queries}.

\subsection{Additional Cross-Embodiment Results: X-Magical \& Kuka Manipulation}
\label{app:cross-domain-results}

Figure~\ref{fig:xmagical_crossdomain_reward} shows the rewards over time for the three cross-embodiment video observations (marked as preferred by the end-user’s ground-truth reward or disliked) in the avoid (left) and group task (right). Across all examples, \rapl’s rewards are highly correlated with the \gt rewards even when deployed on a cross-embodiment robot. 

\begin{figure*}[h!]
    \centering
    \includegraphics[width=\textwidth]{figs/xmagical_crossdomain_reward_new.pdf}
    \caption{\textbf{Cross-Embodiment: X-Magical.} \rapl can distinguish preferred and disliked videos in the cross-embodiment setting. }
    % \vspace{-2em}
\label{fig:xmagical_crossdomain_reward}
\end{figure*}

Figure~\ref{fig:kuka_cross_domain_reward} shows the rewards over time for the two cross-embodiment video observations (marked as preferred by the end-
user’s ground-truth reward or disliked). Across all examples, \rapl’s rewards are highly correlated with the \gt rewards even when deployed on a cross-embodiment robot.

\begin{figure*}[h!]
    \vspace{-0.5cm} 
    \centering
    \includegraphics[width=\textwidth]{figs/robot_kuka_reward_new.pdf}
    \caption{\textbf{Cross-Embodiment: Manipulation.}
    (center) Expert video on \textit{Franka} robot, preferred video on \textit{Kuka}, and disliked \textit{Kuka} video demo. 
    (left) Reward associated with each video under each method. RAPL’s predicted reward generalizes to the \textit{Kuka} robot and follows the GT pattern.
    (right) OT plan for each representation. Columns are embedded frames of expert demo on \textit{Franka} robot. Rows of top matrices are embedded frames of preferred demo on \textit{Kuka}; rows of bottom matrices are embedded frames of disliked demo on \textit{Kuka}. Peaks exactly along the diagonal indicate that the frames of the two videos are aligned in the latent space; uniform values in the matrix indicate that the two videos cannot be aligned (i.e., all frames are equally ``similar’’ to the next). RAPL matches this structure: diagonal peaks for expert-and-preferred and uniform for expert-and-disliked, while baselines show diffused values no matter the videos being compared.}
    \vspace{-0.1cm}
    \label{fig:kuka_cross_domain_reward}
\end{figure*}



\rb{
% \subsection{Additional visual reward baselines in robot manipulation environment}
% \label{app:additional baselines}

% \begin{figure*}[t]
%     \centering
%     \includegraphics[width=\textwidth]{figs/fanka_kuka_new_baselines.pdf}
%     \caption{\rb{\textbf{Manipulation}. Success rate during
% robot policy learning for each visual reward. (left) In-domain experiment. (right) Cross-embodiment experiment.}}
%     \vspace{-0.3cm}
%     \label{fig:new_baseline}
% \end{figure*}

% In addition to \rlhf, \mvpot and \tccot, we added three additional OT-based reward baselines to compare with \rapl in the robot manipulation task described in \autoref{subsubsec:manipulation-setup}: (1) \mvpotfinetune, which fine-tunes MVP representation  using images from the task environment; (2) \rtm, which is an off-the-shelf ResNet-18 encoder \citep{nair2022r3m} pre-trained on the Ego4D data set \citep{grauman2022ego4d} via a learning objective that combines time contrastive learning, video-language alignment, and a sparsity penalty; (3): \imagenet, which is a ResNet-18 encoder pre-trained on ImageNet.

% In Figure~\ref{fig:new_baseline} we show the policy evaluation history during RL training with each reward function. We see \rapl significantly outperforms the new baselines while all baselines struggle to achieve a success rate of more than $\approx 5\%$ with the same number of epochs.


\subsection{Additional complex robot manipulation task with visual distractors}
\label{app: multi object push}

\begin{figure*}[h!]
    \centering
    \includegraphics[width=\textwidth]{figs/fanka_push_multi_objs.pdf}
    \caption{\rb{\textbf{Clutter task: Complex robot manipulation with visual distractors}. (left) Visualization of preferences. Green (preferred behavior): the Franka arm grasps the green rectangular prism and uses that to push the red rectangular prism to the goal region. Red (negative behavior): the Franka arm fails to grasp the rectangular prism. (right) Policy training results for our method and additional baselines.}}
    \vspace{-0.3cm}
    \label{fig:franka_multi}
\end{figure*}



In this section, we consider a more complex robot manipulation task to further validate \rapl's ability to disentangle visual features that underlie an end-user's preferences. 
% from visual input. 
% in a more complex environment. 
We increase the difficulty of the the robot manipulation environment described in \autoref{subsec:in-domain-manipulation} by adding visual distractors that are irrelevant to the human's preferences (left figure in Figure~\ref{fig:franka_multi}). 
The environment has multiple objects on the table of various colors---red, green, and goal-region-blue---and some of the objects are cubes while others are rectangular prisms.
The Franka robot arm needs to learn that the end-user prefers to push the \textit{rectangular} objects (instead of the cubes) \textit{efficiently together} (instead of one-at-a-time) to the goal region. 
% Here, the color of the objects is a visual distractor and is irrelevant to the person's preference. 


\textbf{Task Complexity \& Feature Entanglement.} Compared to the manipulation task described in \autoref{subsec:in-domain-manipulation}, the Franka arm needs to learn representations that can disentangle both semantic preference (grouping) and low-level preference (shape) from RGB images under visual distractors (object color). In addition, the Franka arm needs to learn to \textit{grasp} the rectangular prism first and use that to push the second rectangular prism, as it is difficult to directly push the rectangular prism stably using the robot finger gripper, thus increasing the task difficulty.


\textbf{Privileged State \& Reward.}
The state $s$ is 34D: robot proprioception ($\theta_{\mathrm{joints}}\in \mathbb{R}^{10}$), 3D object positions
($p_{\mathrm{obj_{rect}^{1,2}}}, p_{\mathrm{obj_{cube}^{1,\dots,4}}}$), and object distances to goal ($d_{\mathrm{goal2obj_{rect}^{1,2}}}, d_{\mathrm{goal2obj_{cube}^{1,\dots,4}}}$). The simulated human's reward is:
\begin{align*}
    \rewh_{\mathrm{group}}(s) &= - \max(d_{\mathrm{goal2obj^{rect,1}}}, d_{\mathrm{goal2obj^{rect,2}}}) - ||p_{\mathrm{obj_{rect}^{1}}} - p_{\mathrm{obj_{rect}^{2}}}||_2 \\ &\quad\quad - 0.1 \sum_{i=1}^{4} ||p_{\mathrm{obj_{cube}^{i}}} - p_{\mathrm{obj_{cube}^{i, init}}}||_2.
\end{align*}




\textbf{Baselines.} In addition to comparing \rapl against (1) \gt and (2) \rlhf, we ablate the \textit{representation model} but control the \textit{visual reward structure}. We consider four additional baselines that all use an optimal transport-based reward but operate on different representations: (3): \mvpot which is a off-the-shelf visual transformer \citep{xiao2022masked} pre-trained on the Ego4D data set \citep{grauman2022ego4d} via masked visual pre-training; (4): \mvpotfinetune which fine-tunes \mvpot using images from the task environment via LoRA \citep{hu2021lora}; (5): \rtm which is an off-the-shelf ResNet-18 encoder \citep{nair2022r3m} pre-trained on the Ego4D data set \citep{grauman2022ego4d} via a learning objective that combines time contrastive learning, video-language alignment, and a sparsity penalty; (6): \imagenet which is an off-the-shelf ResNet-18 encoder pre-trined on ImageNet. We use the same preference dataset with $150$ triplets for training RLHF and RAPL. 

\textbf{Results.} The right plot in Figure~\ref{fig:franka_multi} shows the policy evaluation history during RL training with each reward function. We see \rapl performs comparably to \gt (succ. rate: $\approx 65\%)$ while all baselines struggle to achieve a success rate of more than $\approx 10\%$ with the same number of epochs.

}

% \rb{
% \subsection{Spearman’s correlation between GT and learned visual rewards}
% \label{app: reward analysis}

% In this section, we conduct a quantitative analysis to investigate the relationship between the learned visual reward and the end-user’s ground-truth reward. Specifically, for each robot manipulation task, we compute the average Spearman’s correlation coefficient between the learned visual reward and the end-user’s ground-truth reward across 100 video trajectories. We can observe from Table~\ref{table:Spearman} that our learned visual reward shows a stronger correlation to the end-user’s ground-truth reward compared to baselines.
% {
% \renewcommand{\arraystretch}{1.5}
% \begin{table}[h!]
%     \centering
%     \begin{tabular}{p{0.6in}|c | c | c}
%        & \multicolumn{3}{|c}{ \textbf{Spearman's Correlation} } \\ \hline 
%          & \textbf{Franka Group} (Sec.~\ref{subsec:in-domain-manipulation}) & \textbf{Kuka Group} (Sec.~\ref{app:cross-domain-results}) & \textbf{Franka Clutter} (Sec.~\ref{app: multi object push}) \\\hline\hline 
%         \rapl & 0.59 &  0.47 & 0.61\\ \hline
%         \rlhf & 0.38 &  0.31 & 0.26\\ \hline
%         \mvpot &  -0.1&  0.02 & 0.08\\ \hline
%         \mvpotfinetune &  0.19&  0.02& 0.11 \\ \hline
%         \imagenet &  -0.09 &  0.12 & -0.02\\\hline
%         \rtm & 0.03 &  -0.14 &  -0.17 \\ \hline
%     \end{tabular}
%     \caption{\rb{Spearman's rank correlation coefficient between the \gt reward and each learned reward.}}
%     \label{table:Spearman}
% \end{table}
% }
% }

\newpage

\rb{
\subsection{Robot Manipulation: RLHF Perceived vs. True Success}
}

\begin{wrapfigure}{r}{0.4\textwidth}
    \vspace{-0.5cm} \includegraphics[width=0.4\textwidth]{figs/franka_sr_v_learnedreward_rlhf.pdf}
    \vspace{-0.8cm}
    \caption{\rb{\textbf{Manipulation.} True success rate of the RLHF policy (purple) versus the ``perceived'' performance under the RLHF reward (black).}}
    \label{fig:franka_sr_v_learnedreward_rlhf}
    \vspace{-0.2cm}
\end{wrapfigure}
\textcolor{black}{We investigated if the poor RLHF performance in Figure~\ref{fig:franka_success_v_reward} can be attributed to poor RL optimization or to poor visual reward structure. 
We compared the true success rate of the RLHF policy (under the true human’s measure of success) to the ``perceived'' performance under the RLHF reward. 
These results are visualized in Figure~\ref{fig:franka_sr_v_learnedreward_rlhf}: purple is the true success rate and black is the ``perceived'' reward under the RLHF learned reward.
We see that after 350 epochs, the RLHF learned reward perceives the policy as achieving a high reward. However, as shown in the manuscript’s Figure~\ref{fig:franka_success_v_reward} and in Figure~\ref{fig:franka_sr_v_learnedreward_rlhf}, the true success rate is still near zero. This indicates that the RL optimization is capable of improving over time, but it is optimizing a poor reward signal that does not correlate with the true measure of success.
}




% \subsection{The attention map visualization method}

% We visualize the attention map with a novel use of \textit{linear permutation} and \textit{kernel inflation} \citep{xu2022image2point}. Specifically, we use channel-averaged 2D feature map (\textit{i.e.,} activation map) as our attention map \citep{xu2020squeezesegv3}. Different from previous works that operate 2D feature maps, our approach utilizes a linear mapping $\mathcal{W} \in \mathcal{R}^{C_{in} \times C_{out}}$ on a 1D feature, which is average-pooled from a 2D feature $\mathcal{F}_{2D} \in \mathcal{R}^{C_{in} \times H \times W}$. Mathematically, the procedure can be formulated as
% \begin{equation}
%     \hat{\mathcal{F}}_{1D} = \frac{\mathcal{W}^T \times \sum_i^{H \times W}\mathcal{F}_{2D}^i}{H \times W}
% \end{equation}
% where $\hat{\mathcal{F}}_{1D} \in \mathcal{R}^{C_{out} \times 1}$ is the adapted features from our proposed RAPL by $\mathcal{W} \in \mathcal{R}^{C_{in} \times C_{out}}$. Inspired by \cite{xu2022image2point}, we can inflate the 1D linear mapping $\mathcal{W} \in \mathcal{R}^{C_{in} \times C_{out}}$ into 2D and keep the kernel size as 1, \textit{i.e.}, $\mathcal{W} \in \mathcal{R}^{C_{in} \times C_{out}} \rightarrow \mathcal{W}_{inflate} \in \mathcal{R}^{C_{in} \times C_{out} \times 1 \times 1}$. Then above equation can be equally represented as 
% \begin{equation}
%      \hat{\mathcal{F}}_{2D}  = \mathcal{W}_{inflate}^T \times \mathcal{F}_{2D}, 
%      \hat{\mathcal{F}}_{1D} = \frac{\sum_i^{H \times W}\hat{\mathcal{F}}^i_{2D}}{H \times W}
% \end{equation}
% We average the $\hat{\mathcal{F}}_{2D} \in \mathcal{R}^{C_{out} \times H \times W}$ in channel dimension, and visualize the output as our attention map.
